# Supplementary material for: Off Environment Evaluation Using Convex Risk Minimization
Source: arXiv:2112.11532 source file (2021-12-21)
Supplement: Supplementary file 1 [file appendix.tex]

\section{Supplementary Material}
\subsection{Theorem 5.1}
The Kullback-Leiber divergence between two distributions $P$ and $Q$ can be rewritten as a maximisation problem over a space of functions $\mathcal{G}$ ~\cite{DBLP:journals/tit/NguyenWJ10}:
\begin{align}\label{eq: expoptimizer}
\begin{split}
    &\hat{\mathcal{D}}_{KL}(P || Q) =\\
    -&\left (\min_{g \in \mathcal{G}} \sum_{x \in \Omega} Q(x) g(x) 
    -\sum_{x' \in \Omega}P(x') \log(g(x')) -  1\right)  \\
    &= \min_{g \in \mathcal{G}} L(g)
    \end{split}
\end{align}
Note that the optima of the above problem is $g^*= \frac{P(x)}{Q(x)}$, as desired. In practice we only have access to $n$ samples each from $P$ and $Q$, the optimal $g^*$ is approximated by searching for $\hat{g}_n$ that minimizes the empirical loss along with a regularizer $I(g)$ to prevent over-fitting:
\begin{align}\label{eq: optimizer}
    \hat{g}_n = \arg \min_{g \in \mathcal{G}}
    \frac{1}{n}\sum_{i=1}^n g(x_i') - \frac{1}{n}\sum_{i=1}^n \log(g(x_i)) + \frac{\lambda_n}{2} I(g)^2
\end{align}
For implementation purposes we make sure that the space of functions $\mathcal{G}$ satisfies the following assumptions. 
\begin{assumption}\label{ass: bounds}
For any $g \in \mathcal{G}$, we assume that $\nu \leq g(x) \leq \mu \quad \forall x \in \Omega$. Note that $\nu < 1$ and $\mu > 1$
\end{assumption}
\begin{assumption}\label{ass: existence}
$\exists$ $g^* \in \mathcal{G}$ such that $g^*(x) = \frac{P(x)}{Q(x)}$
\end{assumption}
For the sake of simplicity we are also going to assume that $\mathcal{G}$ contains the true minimizer $g^*$. 
Under these assumptions we can analyze the error between the empirically estimated optimizer $\hat{g}_n$ and the true optimizer $g^*$ as follows, 

\textbf{Theorem 5.1} Under assumption \ref{ass: bounds} and \ref{ass: existence}, we can upper bound the estimator error $\hat{g}_n$ and $g^*$, with probability at-least $1- \delta$ and for a sufficiently large $n$ by,
\begin{align}\label{eq: upperbound}
\begin{split}
&\| \hat{g}_n - g^* \|_\infty^2 \leq \\&
Ke^{D_{\infty}(P \| Q)}(\sqrt{\frac{1}{n}}  (\mu  + \max(\log(\mu), -\log(\nu)) \\ &+ \sqrt{2 \log(\frac{1}{\delta})}) \\
\end{split}
\end{align}
For the sake of simplicity we abbreviate the upper-bound as as a function of the function class $\mathcal{G}$ and $\delta$ as $M(\mathcal{G}, \delta)$. 
\subsection{Proof of Theorem 5.1}\label{sec: error}
Since, equation \ref{eq: optimizer} is an empirical form of equation \ref{eq: expoptimizer} it is an Empirical Risk Minimization algorithm. We denote the original loss with respect to a function $g \in \mathcal{G}$ as $L(g)$.  Using familiar result from learning theory (Corollary 6.1 ~\cite{DBLP:journals/corr/Hajek}) with probability at-least $1-\delta$
\begin{align}
    L(\hat{g}_n) - L(g^*) \leq 4 \mathbb{E} \mathcal{R}_n(\mathcal{G}(X^n, Y^n)) + \sqrt{\frac{2 \log(\frac{1}{\delta})}{n}} \label{eq: slt}
\end{align}
Where, $\mathcal{R}_n(\mathcal{G}(X^n, Y^n))$ is the Radamacher average such that for $\forall \varepsilon_i$ is binomial distribution distributed uniformly in $\{-1, 1\}$. 
\begin{align}
    \mathcal{R}_n(\mathcal{G}(X^n, Y^n)) &= \frac{1}{n} \mathbb{E}_{\varepsilon^n} [\sup_{g \in \mathcal{G}} |\sum_{i} \varepsilon_i (g(x_i) - \log(g(y_i)|] 
\end{align}
Using the fact that the points $x_i \sim Q$ and $y_i \sim P$ are independent from each other. Using Jensen's inequality for a convex function $\phi(x)$, $\phi(\mathbb{E}[x]) \leq \mathbb{E}[\phi(x)])$. Using the fact that $\varepsilon_i$'s are independent of each other. 
\begin{align}
\begin{split}
    &\mathcal{R}_n(\mathcal{G}(X^n, Y^n)) = \frac{1}{n} \mathbb{E}_{\varepsilon^n} [\sup_{g \in \mathcal{G}} |\sum_{i} \varepsilon_i (g(x_i) - \log(g(y_i)|] \\
    &\leq \frac{1}{n} \mathbb{E}_{\varepsilon^n} \sup_{g \in \mathcal{G}} \sum_i |\varepsilon_i g(x_i) | +  \sup_{g \in \mathcal{G}} \sum_i |\varepsilon_i \log(g(y_i)) | \\
    &\leq \frac{1}{n} (\sqrt{\sum_i g(x_i)^2 } + \sqrt{\sum_i log(g(y_i))^2 })\\
    &\leq \sqrt{\frac{1}{n}} (\mu + max(\log(\mu), -\log(\nu)) \label{eq:error_bound}
    \end{split}
\end{align}
The last set of inequality comes from assuming that $ g(x) \in [\nu, \mu]$ $\forall g \in \mathcal{G}, \forall x \in \Omega$. And the fact that $\nu \in (0, 1)$ and  $\mu \geq 1$. Using equation \ref{eq:error_bound} in equation \ref{eq: slt} we get, 
\begin{align}\label{eq: radaapprox}
\begin{split}
    &L(\hat{g}_n) - L(g^*) \leq \\
    &4 \sqrt{\frac{1}{n}} \left(\mu + \max(\log(\mu), -\log(\nu)) + \sqrt{ 2\log(\frac{1}{\delta})}\right)
    \end{split}
\end{align}
With probability at least $1-\delta$. Now, let's turn our attention to the left hand side. Before we end up doing that let's define the estimation error $\Bar{e}_n(x) = \hat{g}_n(x) - g^*(x)$. Thus, we can re-write the left hand side in terms of $\Bar{e}$
\begin{align}
\begin{split}
    L(\hat{g}_n) - L(g^*)  &= L(g^* + \Bar{e}_n) - L(g^*)\\
    &= \sum_{x \in \Omega} Q(x) \bar{e}_n -\sum_{x \in \Omega} P(x) log(\frac{\Bar{e}_n + g^*}{g^*}) \\
    &= \sum_{x \in \Omega} Q(x) (\bar{e}_n - g^* \log(1 + \frac{\bar{e}_n}{g^*})) 
    \end{split}
\end{align}
Assuming that $n$ is sufficiently large such that $|\frac{\Bar{e}_n}{g^*}| \leq 1$. We can now use second order Taylor approximation for $\log (1 + x)$ for $|x| < 1$
\begin{align}\label{eq:taylorapprox}
\begin{split}
     L(\hat{g}_n) - L(g^*)  &= \sum_{x \in \Omega} Q(x) (\Bar{e}_n - g^*( \frac{\Bar{e}_n}{g^*} - \frac{1}{2} (\frac{\Bar{e}_n}{g^*})^2)) \\
     &= \sum_{x \in \Omega} Q(x)\frac{1}{2}(\frac{\Bar{e}_n^2}{g^*})
     \end{split}
\end{align}
Combining equations \ref{eq: radaapprox} and the above equation, we can bound the error with probability at least $1-\delta$ that, 

\begin{align}
\begin{split}
\sum_{x \in \Omega} &Q(x)\frac{1}{2}(\frac{\Bar{e}_n^2}{g^*}) \leq\\
&4 \sqrt{\frac{1}{n}} \left 
(\mu + \max(\log(\mu), -\log(\nu)) + \sqrt{2 \log(\frac{1}{\delta})} \right)
\end{split}
\end{align}
Under assumption \ref{ass: bounds} and \ref{ass: existence} $\exists x^* \in \Omega$ such that $|\bar{e}_n(x^*)| =  \| \hat{g}_n - g^*\|_\infty$. Thus, the equation above can be re-written as 
\begin{align}
\begin{split}
    &\frac{1}{K }\| \Bar{e}_n \|_\infty^2 \leq  \\
    &8 g^*\sqrt{\frac{1}{n}} \left (\mu + \max(\log(\mu), -\log(\nu)) + \mu \sqrt{2 \log(\frac{1}{\delta})}\right) \\
    &8 e^{D_{\infty(P \| Q)}}\sqrt{\frac{1}{n}} \left(\mu + \max(\log(\mu), -\log(\nu)) + \mu \sqrt{2 \log(\frac{1}{\delta})}\right)
    \end{split}
\end{align}
where $Q(x^*) = \frac{1}{K}$. The last inequality comes from the fact that $g^*(x^*) = \frac{P(x)}{Q(x)} \leq \sup_{x \in \Omega} \frac{P(x)}{Q(x)} = e^{D_{\infty} (P \| Q)}$. 
This completes the proof. 
\section{Estimating $\zeta$}
Using this theorem, we now bound the error in estimation of $\zeta$
\begin{align}\label{eq: zeta}
    \zeta(s' | s, a) = \Large \left({\frac{d^{\mathcal{D}_{te}}(s, a, s')}{d^{\mathcal{D}_{tr}}(s, a, s')}}\Large\right)\bigg/ \large \left({\frac{d^{\mathcal{D}_{te}}(s, a)}{d^{\mathcal{D}_{tr}}(s, a)}} \large \right)
\end{align}
Note that $\zeta$ estimation requires taking a ratio of two such aforementioned estimations. Since, each of these estimations are error prone, it also adds to error of estimating $\zeta$. We first take note of the following lemma from numerical analysis~\cite{numericalanalysis}
\begin{lemma}\label{le: product}
    Consider the following the function $f(x_1, x_2, ..., x_n) = \Pi_{i=1}^n x_i$. Now, instead of actual values of $x_i$'s suppose we have noisy estimates $x_i' = x_i + \varepsilon_i$. Using familiar results from numerical analysis, we can bound the first order error between the noisy estimate and the actual value as follows, 
\begin{align}
\begin{split}
    &| f(x_1', x_2', x_3', ..., x_n') - f(x_1, x_2, ..., x_n)| \\ &\leq {f(x_1, x_2, ..., x_n)} \sum_{i=1}^n \frac{\varepsilon_i}{x_i} \\
    & x_i \neq 0 \quad\forall i \in \{1,2,3,..., n\} 
    \end{split}
\end{align}
\end{lemma}
\begin{proof}
Let us first calculate what $| f(x_1', x_2', x_3', ..., x_n') - f(x_1, x_2, ..., x_n)|$ looks like
\begin{align}
\begin{split}
    &| f(x_1', x_2', x_3', ..., x_n') - f(x_1, x_2, ..., x_n)| \\&= 
    \sum_{i=1}^n \left ( \prod_{j \neq i } x_j \right)  \varepsilon_i  + O(\varepsilon^2)\\
    &\leq\sum_{i=1}^n \left ( \prod_{j } x_j \right)  \frac{\varepsilon_i}{x_i} \\
        &\leq \left ( \prod_{j } x_j \right)  \sum_{i=1}^n  \frac{\varepsilon_i}{x_i}  = f(x_1, x_2, ..., x_n) \sum_{i=1}^n  \frac{\varepsilon_i}{x_i}
    \end{split}
\end{align}
This completes the proof. 
\end{proof}
Using the above lemma along with theorem \textit{5.1} we now propose the error bound for estimating $\zeta$. 
\begin{lemma}\label{le: zetaerror}
Applying theorem 5.1 and lemma \ref{le: product} we can bound estimation error for $\hat{\zeta}_n$ as follows, 
\begin{align}
    \| \hat{\zeta}_n - \zeta^* \| &\leq \frac{\mu(1 + \nu \mu)}{\nu^2} \frac{M(\mathcal{G}, \delta)}{n^{1/4}}
\end{align}
\end{lemma}
\begin{proof}
Assuming that the $\zeta$ estimation can be written in functional form as follows, 
\begin{align}
\begin{split}
    &f({\frac{d_{\mathcal{P}_{te}}^\pi(s, a, s')}{d_{\mathcal{P}_{tr}}^\pi(s, a, s')}},{\frac{d_{\mathcal{P}_{tr}}^\pi(s, a)}{d_{\mathcal{P}_{te}}^\pi(s, a)}}) \\
    &= \left({\frac{d_{\mathcal{P}_{te}}^\pi(s, a, s')}{d_{\mathcal{P}_{tr}}^\pi(s, a, s')}}\Large\right) \large \left({\frac{d_{\mathcal{P}_{tr}}^\pi(s, a)}{d_{\mathcal{P}_{te}}^\pi(s, a)}} \large \right)
    \end{split}
\end{align}
We can now apply lemma \ref{le: product} along with theorem 5.1 which completes the proof. 
\end{proof}
Using the bounds on the estimation of $\hat{\zeta}_n$. We now prove the error bound in on the evaluation of returns $ {J_{\mathcal{P}_{te}}(\pi)}$
\section{Theorem 5.2}
In this section, we wish to bound the error in evaluation using the estimator that we calculated using equation \ref{eq: zeta}.  Using this calculated $\hat{\zeta}_n$, we evaluate returns (equation \ref{eq:jzetan}). To analyse the error we again re-define these two terms. 
\begin{flalign}
   J_{\mathcal{P}_{te}}(\pi)  &=  \mathbb{E}[\sum_{t=0}^{T} \gamma^t \prod_{k=1}^t \zeta(s_{k-1}, a_{k-1}, s_k) r(s_t, a_t) ]\\
   J_{\mathcal{P}_{te}}^{\hat{\zeta}_n}(\pi)  &=  \mathbb{E}[\sum_{t=0}^{T} \gamma^t \prod_{k=1}^t \hat{\zeta}_n(s_{k-1}, a_{k-1}, s_k) r(s_t, a_t) ] \label{eq:jzetan}\\
    & a_t = \pi(s_t) \quad s_{t+1} \sim \mathcal{P}_{tr}(.|s_t, a_t) \quad s_0 \sim S_0 \nonumber
\end{flalign}
\textbf{Theorem 5.2}
Under assumptions \ref{ass: existence} and \ref{ass: bounds} and the assumption that the reward function is bounded by a constant $\|r(s,a)\|_\infty \leq R$, we can bound $|J_{\mathcal{P}_{te}}(\pi)  - J_{\mathcal{P}_{te}}^{\hat{\zeta}_n}(\pi)|^2$ with atleast $1-\delta$ probability: 
\begin{align}
\begin{split}
    &|J_{\mathcal{P}_{te}}(\pi)  - J_{\mathcal{P}_{te}}^{\hat{\zeta}_n}(\pi)|^2 \\
    &\leq \frac{TM (\mathcal{G}, \delta)^2 R^2 \gamma }{\nu \sqrt{n}} \left(\frac{1 - (T+1)\frac{\gamma}{\nu}^T + T\frac{\gamma}{\nu}^{T+1}}{(1 - \frac{\gamma}{\nu})^2} \right)
    \end{split}
\end{align}

\begin{proof}
In order to estimate error, we first use the triangular inequality to divide the left hand side into terms dependent on a particular time instant.
\begin{align}
\begin{split}
     & |J_{\mathcal{P}_{te}}(\pi)  -  J_{\mathcal{P}_{te}}^{\hat{\zeta}_n}(\pi)| ^2 \\
    &=  |\mathbb{E}[\sum_{t=1}^T \gamma^t \Pi_{k=1}^{t-1}  (\zeta^*(s_{k-1}, a_{k-1}, s_{k}) \\
    & - \hat{\zeta}_n(s_{k-1}, a_{k-1}, s_{k}))  r(s_t, a_t) ]\|_\infty^2 \\
    &\leq T (\sum_{t=1}^T \mathbb{E}[\gamma^t \Pi_{k=1}^{t-1} (\zeta^*(s_{k-1}, a_{k-1}, s_{k}) \\
    & - \hat{\zeta}_n(s_{k-1}, a_{k-1}, s_{k}))  r(s_t, a_t)])^2
    \end{split}
\end{align}
where, the last inequality follows from applying the triangular inequality. We complete the proof by using lemma \ref{le: product} along with lemma \ref{le: zetaerror} to upper-bound each of these terms as follows, 
\begin{align}
\begin{split}
   &|J_{\mathcal{P}_{te}}(\pi)  - J_{\mathcal{P}_{te}}^{\hat{\zeta}_n}(\pi)|_\infty ^2 \\
   &\leq T \sum_{t=1}^T ((\gamma \frac{\mu}{\nu})^t \frac{\mu(1 + \nu \mu)}{\nu^2} \frac{M(\mathcal{G}, \delta)}{n^{1/4}}tR)^2 \\
    &\leq (\frac{\mu^2(1 + \nu \mu)^2}{\nu^4})\frac{TM(\mathcal{G}, \delta)^2 R^2}{\sqrt{n}} \sum_{t=1}^T (\frac{\gamma \mu}{\nu})^t t  \\
    &\leq  (\frac{\mu^2(1 + \nu \mu)^2}{\nu^4})\frac{TM(\mathcal{G}, \delta)^2 R^2}{\sqrt{n}} \times \\
&    (\frac{1 - T(\frac{\gamma \mu}{\nu})^T}{1 - \frac{\gamma \mu }{\nu}} + \frac{\frac{\gamma \mu }{\nu}(1 - (\frac{\gamma \mu}{\nu})^{T-1}) }{(1 - \frac{\gamma \mu}{\nu})^2}) \nonumber \\
    \end{split}
\end{align}
where the last inequality comes from applying the sum of Arithmetic Geometric Progression (AGP) series which completes the proof.  
\end{proof}
\section{Implementation Details}
For all the experiments, we keep our class of classifiers as a 3-layered neural network with relu based activation function. The final output has a tanh layer, which is scaled to $[\nu, \mu]$ (Assumption \ref{ass: bounds}). The network was trained using data from both the training and testing MDP using a stochastic gradient descent algorithm with $10^{-5}$ learning rate. 

Using data from the testing MDP $\mathcal{D}^{te}$ along with the training MDP $\mathcal{D}^{tr}$, we train two network using the equation \ref{eq: optimizer}. One, where we sample the state-action pairs $\{(s, a)\}_{te} \sim \mathcal{D}^{te},\{(s, a)\}_{tr }\sim \mathcal{D}^{tr}$ to calculate the state-action density ratio between testing and the training MDP. Two, where we sample state-action-state tuples $\{(s, a, s')\}_{te} \sim \mathcal{D}^{te}, \{(s, a, s')\}_{tr} \sim \mathcal{D}^{tr}$ to calculate state-action-state density ratio between two MDPs. We recall the definition of state-action density and state-action-state density with respect to a policy $\pi$ below
\begin{align}\label{eq: stationarydist}
\begin{split}
    &d_{\mathcal{P}}^\pi(s, a) = (1-\gamma) \sum_{t=0}^\infty \gamma^t \mathcal{P}r(s_t = s, a_t = a) \\
    &d_{\mathcal{P}}^\pi(s, a, s') = (1-\gamma) \sum_{t=0}^\infty \gamma^t \mathcal{P}r(s_t = s, a_t = a, s_{t+1} = s') \\
   & s_0 \sim S_0 \quad a_t \sim \pi(.|s_t) \quad s_{t+1} \sim \mathcal{P}(.|s_t, a_t)
    \end{split}
\end{align}

We further exploit the relationship $
    d_{\mathcal{P}}^\pi(s, a, s') = d_{\mathcal{P}}^\pi(s, a) \mathcal{P}(s'|s, a)$  between these two trained networks to calculate $\zeta$ (equation \ref{eq: zeta})

For the purpose of experiments, we assumed that one of the simulation parameters as the training MDP and use different testing MDPs over which to test our approach. For example, for the cartpole set of experiments we keep gravity value $g = 10.0 m/s^2$ as the training MDP, the results are evaluated on a range of different testing MDPs which are parameterised by gravity $g$. 

Specifically for the cartpole set of experiments, we also add a small amount of gaussian noise with standard deviation $10^{-3}$ to keep things in line with the assumption \ref{ass: bounds} and \ref{ass: existence}. 
\subsection{Estimating $\beta$}\label{sec: beta}
\begin{figure*}[!ht]
\centering
\begin{minipage}{0.23 \textwidth}
\subfigure[$P \sim \mathcal{N}(2, 1)$  ]{\label{fig:betahat1}\scalebox{0.4}{\hbox{\input{Beta/beta_2142}}}}
\end{minipage}%
\begin{minipage}{0.23\textwidth}
\subfigure[$P \sim \mathcal{N}(3, 1)$ ]{\label{fig:betahat2}\scalebox{0.4}{\hbox{\input{Beta/beta_3142}}}}
\end{minipage}%
\begin{minipage}{0.23\textwidth}
\subfigure[$P \sim \mathcal{N}(4, 1)$]{\label{fig:betahat3}\scalebox{0.4}{\hbox{\input{Beta/beta_4142}}}}
\end{minipage}
\caption{Estimating $\beta = \frac{P(x)}{Q(x)}$ for two normal distributions with $Q \sim \mathcal{N}(4, 2)$}
\end{figure*}
We evaluate the effectiveness of the estimator to calculate the ratio of probability distributions using sampled points from two different distributions $p$ and $q$. To that end, we minimize the loss function mentioned in \ref{eq: optimizer} where the optimizer would be the estimated ratio of probability distributions. We report performance for three pairs of normal distributions $p, q$ over different sample sizes used to train for this ratio. Our results are presented in figures \ref{fig:betahat1}, and \ref{fig:betahat2} and \ref{fig:betahat3}. We observe that when the two distributions are similar (figure \ref{fig:betahat3}) the estimator learns the ratio much more quickly as compared to the case when the divergence is more (figure \ref{fig:betahat1}). For example, 2000 samples is good enough to give a good enough estimate of the ratio when the distributions are closer. However, as the divergence between two distributions increases, we require larger sample sizes to get a reasonable estimate of the density ratio.
\subsection{Archery Environment}
\begin{figure*}
\centering
\begin{minipage}{.23\textwidth}
\centering
\subfigure[$W_{te} \sim \mathcal{N}(2,1)$]{\label{fig:dartenv_2}\scalebox{0.4}{\hbox{\input{DartEnv/dart_evaluation_2142}}}}
\end{minipage}
\begin{minipage}{.23\textwidth}
\centering
  \subfigure[$W_{te} \sim \mathcal{N}(3,1)$]{\label{fig:dartenv_3}\scalebox{0.40}{\hbox{\input{DartEnv/dart_evaluation_3142}}}}
\end{minipage}%
\begin{minipage}{.23\textwidth}
\centering
\subfigure[$W_{te} \sim \mathcal{N}(4,1)$]{\label{fig:dartenv_4}\scalebox{0.4}{\hbox{\input{DartEnv/dart_evaluation_4142}}}}
\end{minipage}%
\begin{minipage}{.23\textwidth}
\centering
\subfigure[Archery \newline  Schematic]{\label{fig:dartenv_schematic}\scalebox{0.4}{\input{DartEnv/dartschematic}}}
\vspace{-7pt}
\end{minipage}
\caption{Off Environment Evaluation for Archery Environments with $MDP_{tr} \sim \mathcal{N}(4,2)$}
\label{fig: dartenv}
\end{figure*}
In this section we demonstrate the ability of our algorithm to estimate the ratio of transition probabilities. We use the archery environment to demonstrate the effectiveness of our approach over a three different pair of environments. \\\\
As shown in the figure \ref{fig:dartenv_schematic} is a schematic of the archery task. The agent has to choose an angle of attack such that it hits the bulls eye which is set at the origin. The arrow faces resistance in form of horizontal wind flow with varying speeds. In these set of experiments, we parameterize the wind with different probability distributions to create different environments. Note that this system acts as a 1-step MDP, because the distribution of final position of the arrow is dependent on the angle of attack. We show that it is possible to compute the ratio of transition probabilities using samples from the two different environment, by evaluating the performance of the target environment by using the training environment and the estimated ratio (equation 4.2).\\\\
For these experiments we used a training environment where the wind speed is sampled from a normal distribution $\mathcal{N}(4, 2)$. Using this training environment we approximate the ratio of transition probabilities for three different target environments. Each of these target environments have horizontal wind speed distributed as $\mathcal{N}(2, 1), \mathcal{N}(3, 1), \mathcal{N}(4, 1)$, respectively. To demonstrate the effectiveness of this approximation, we evaluate the average performance of the agent in the target domain using the simulator and the estimated transition probability ratio. These performance results are plotted against the true performance of the same agent in these target environments. The cost function that we use is the negative of absolute distance of the arrow from the bull's eye (which is the origin). \\\\
The evaluation results for each of these environments are shown in figures \ref{fig:dartenv_2}, \ref{fig:dartenv_3} and \ref{fig:dartenv_4} respectively. We observe that our method in all the three instances was able to approximate performance with very high accuracy. We also observe that the deviations between estimated performance and the true value is larger when the data sampled is sparse. For example, in all the three figures we observe that the error is larger around $\theta = 0.5$.
